# Supplementary material for: A polymer model of bacterial supercoiled DNA including structural transitions of the double helix
Source: arXiv:1904.11453 source file (2019-04-25)
Supplement: Supplementary file 1 [file SI.pdf]

# Supplemental material: A polymer model of bacterial supercoiled DNA including structural transitions of the double helix

Thibaut Lepage and Ivan Junier

*CNRS, TIMC-IMAG, F-38000 Grenoble, France*

*Univ. Grenoble Alpes, TIMC-IMAG, F-38000 Grenoble, France*

**CONTENTS**

I. Supplementary methods 2
A. Derivation of the effective model with a global torsional energy 2
B. Free energy profiles in the zero writhe approximation 4
C. Generalization to an arbitrarily number of alternative forms 5
D. Torques 6
1. Measurement in numerical simulations 6
2. Expression in the zero writhe approximation and access to the torsional modulus 6
E. Inference of parameters by testing a large number of parameters 7
References 7
II. Supplementary figures 9

## I. SUPPLEMENTARY METHODS

In the following, parameters are uniform along the DNA molecule. Sequence effects will be treated in subsequent works.

### A. Derivation of the effective model with a global torsional energy

We start by writing down the equilibrium probability of a configuration $\mathcal{C}$ with DNA-form profile $\{s_i\}_{i=1..N}$ in the context of an imposed linking number Lk. To this end, we divide the conformational energy into two terms: the torsional energy $E_T(\mathcal{C}) = \frac{k_BT}{2}\sum_{i=1}^{N}\frac{nC_{s_i}}{a_{s_i}}(\phi_i-\psi_{s_i})^2$ that depends on the torsional angles $\{\phi_i\}_{i=1..N}$ and the rest, $E_{\overline{T}}(\mathcal{C})$, which does not. In this context, denoting $\beta = 1/k_BT$, we have:

$$P(\mathcal{C}) = Z^{-1}\exp\left[-\beta E_{\overline{T}}(\mathcal{C}) - \sum_i \frac{nC_{s_i}}{2a_{s_i}}(\phi_i-\psi_{s_i})^2\right]\delta\left(\mathrm{Tw}(\mathcal{C}) - \mathrm{Tw}_{\mathrm{Lk}}(\mathcal{C})\right) \quad (1)$$

with $Z$ the partition function such that $\sum_{\mathcal{C}} P(\mathcal{C}) = 1$. The $\delta(x)$ function, which is equal to 1 if $x = 0$ and 0 otherwise, imposes the conservation of Lk, that is, it only retains conformations for which the total twist of the molecule, $\mathrm{Tw}(\mathcal{C})$, is equal to $\mathrm{Tw}_{\mathrm{Lk}}(\mathcal{C}) \equiv \mathrm{Lk} - \mathrm{Wr}(\mathcal{C})$.

Using $\mathrm{Tw}(\mathcal{C}) = (2\pi)^{-1}\sum_i n\phi_i$ and defining $\mathrm{t}(\mathcal{C}) = \mathrm{Tw}_{\mathrm{Lk}}(\mathcal{C})/N_{\mathrm{bp}} = \mathrm{Tw}_{\mathrm{Lk}}(\mathcal{C})/nN$, Eq. 1 can be rewritten as:

$$P(\mathcal{C}) = Z^{-1}\exp\left[-\beta E_{\overline{T}}(\mathcal{C}) - \sum_i \frac{nC_{s_i}}{2a_{s_i}}(\phi_i - \psi_{s_i})^2\right]\delta\left(\sum_i \phi_i - 2\pi\mathrm{t}N\right) \quad (2)$$

The integration over the $\phi_i$'s then results in evaluating the following term (for clarity, we drop the $\mathcal{C}$'s):

$$\begin{aligned}
I = &\int \prod_k d\phi_k \exp\left[-\sum_i \frac{nC_{s_i}}{2a_{s_i}}(\phi_i - \psi_{s_i})^2\right]\delta\left(\sum_i \phi_i - 2\pi\mathrm{t}N\right) = \\
&\text{(using the Fourier transform of } \delta\text{)} \\
&\int dx \prod_k \int d\phi_k \exp\left[-\frac{nC_{s_k}}{2a_{s_k}}(\phi_k - \psi_{s_k})^2 - 2\pi i x(2\pi\mathrm{t} - \phi_k)\right] = \\
&\int dx \prod_k \int d\phi_k \exp\left[-\frac{nC_{s_k}}{2a_{s_k}}\left(\phi_k - \psi_{s_k} - \frac{2\pi i a_{s_k}}{nC_{s_k}}x\right)^2\right]\exp\left[-\frac{2\pi^2 a_{s_k}}{nC_{s_k}}x^2 - 2\pi i x(2\pi\mathrm{t} - \psi_{s_k})\right] = \\
&\left[\prod_k \int d\phi_k \exp\left[-\frac{nC_{s_k}}{2a_{s_k}}\left(\phi_k - \psi_{s_k} - \frac{2\pi i a_{s_k}}{nC_{s_k}}x\right)^2\right]\right]\int dx \exp\left[-\sum_j\left(\frac{2\pi^2 a_{s_k j}}{nC_{s_j}}x^2 + 2\pi i x(2\pi\mathrm{t} - \psi_{s_j})\right)\right] \quad (3)
\end{aligned}$$

Defining the conformation-dependent average torsional susceptibility per base pair $\chi(\mathcal{C}) \equiv \sum_{i=1}^{N}\frac{a_{s_i}}{C_{s_i}}/N$, the conformation-dependent average twist angle at rest $\psi(\mathcal{C}) \equiv \sum_{i=1}^{N}\psi_{s_i}/N$, we obtain (still dropping the $\mathcal{C}$'s):

$$\begin{aligned}
I &= (2\pi)^{N/2}\sqrt{\prod_k \frac{a_{s_k}}{nC_{s_k}}}\int dx \exp\left[-\frac{2\pi^2 N\chi}{n}\left(x^2 + i\frac{n}{\pi\chi}(2\pi\mathrm{t} - \psi)x\right)\right] \\
&= (2\pi)^{N/2}\sqrt{\prod_k \frac{a_{s_k}}{nC_{s_k}}}\int dx \exp\left[-\frac{2\pi^2 N\chi}{n}\left(\left(x + i\frac{n}{2\pi\chi}(2\pi\mathrm{t} - \psi)\right)^2 + \frac{n^2}{4\pi^2\chi^2}(2\pi\mathrm{t} - \psi)^2\right)\right] \\
&= (2\pi)^{N/2}\sqrt{\prod_k \frac{a_{s_k}}{nC_{s_k}}}\exp\left[-\frac{nN}{2\chi}(2\pi\mathrm{t} - \psi)^2\right]\int dx \exp\left[-\frac{2\pi^2 N\chi}{n}\left(x + i\frac{n}{2\pi\chi}(2\pi\mathrm{t} - \psi)\right)^2\right] \\
&= \frac{(2\pi)^{(N-1)/2}}{N^{1/2}}\sqrt{\prod_k \frac{a_{s_k}}{\chi C_{s_k}}}\exp\left[-\frac{nN}{2\chi}(2\pi\mathrm{t} - \psi)^2\right] \\
&= \frac{(2\pi)^{(N-1)/2}}{N^{1/2}}\exp\left[-\frac{1}{2}\left(\frac{N_{\mathrm{bp}}}{2\chi}(2\pi\mathrm{t} - \psi)^2 + \ln(\chi) - \sum_i \ln\left(\frac{a_{s_i}}{C_{s_i}}\right)\right)\right], \quad (4)
\end{aligned}$$

which, after redistribution of the terms $\ln(\chi)$ and $\ln\left(\frac{a_{s_i}}{C_{s_i}}\right)$ in the torsional energy and the free energy of formation, respectively, leads to the effective energies of the main text (Eqs. 3 and 4). Note also that in Eq. 4 of the main text, we have used the fact that $\mathrm{Tw}(\mathcal{C}) = \mathrm{Tw}_{\mathrm{Lk}}(\mathcal{C})$ in the simulated polymer model.

### B. Free energy profiles in the zero writhe approximation

In the case of the co-existence of two forms, here B-DNA and X-DNA (any alternative DNA form), using Eqs. 2, 3 and 4 of the main text, the effective energy, $U(\lambda, X)$, of a conformation where X-DNA occupies $\lambda N$ sites (corresponding to $\lambda N_{\rm bp}$ base pairs) distributed in $X$ domains reads:

$$U(\lambda, X) = \lambda N_{\rm bp}\gamma_X + 2XJ + E_B^X - fz_X + E_B^B - fz_B \\ +\frac{k_BT}{2}\left[\frac{N_{\rm bp}}{\chi(\lambda)}\left(2\pi\frac{\rm Tw}{N_{\rm bp}} - \psi(\lambda)\right)^2 + \ln\left(\chi(\lambda)\right)\right] \quad (5)$$

where $E_B^s$ indicates the total bending energy of the form $s$ and where we have used the notations $\chi_s = a_s/C_s$ and $\chi/\psi(\lambda) = (1-\lambda)\chi_B/\psi_B + \lambda\chi_s/\psi_s$ – note that $\psi(\lambda)$ represents the average twist angle at rest of the molecule with a fraction $\lambda$ of alternative forms. Next, considering that the supercoiling density, $\sigma$, is totally converted into twist in the approximation of zero writhe, we can replace $2\pi\frac{\rm Tw}{N_{\rm bp}}$ by $(1+\sigma)\psi_B$. Finally, integrating the corresponding partition function over the bending angles of each site leads to a free energy where the terms $E_B^s - fz_s$ are replaced by $g_{s,f}(X)$, the free energy associated with the WLC at force $f$ with bending modulus $K_s$ and contour length $X$. The resulting bi-dimensional free energy surface, $S_{f,\sigma}(\lambda, X)$ therefore reads:

$$S_{f,\sigma}(\lambda, X) = \lambda N_{\rm bp}\gamma_X + 2XJ + g_{X,f}(\lambda N_{\rm bp}a_X) + g_{B,f}((1-\lambda)N_{\rm bp}a_B) + \\ \frac{k_BT}{2}\left[\frac{\psi_B^2 N_{\rm bp}}{\chi(\lambda)}\left(1+\sigma-\frac{\psi(\lambda)}{\psi_B}\right)^2 + \ln\left(\chi(\lambda)\right)\right] \quad (6)$$

The unidimensional free energy profile $F_{f,\sigma}(\lambda)$ (Eq. 5 in the main text) can be obtained by summing (with Boltzmann weights) over the values of $X$, leading to:

$$F_{f,\sigma}(\lambda) = \lambda N_{\rm bp}\gamma_X + \mathcal{J}(\lambda) + g_{X,f}(\lambda N_{\rm bp}a_X) + g_{B,f}((1-\lambda)N_{\rm bp}a_B) + \\ \frac{k_BT}{2}\left[\frac{\psi_B^2 N_{\rm bp}}{\chi(\lambda)}\left(1+\sigma-\frac{\psi(\lambda)}{\psi_B}\right)^2 + \ln\left(\chi(\lambda)\right)\right] \quad (7)$$

with:

$$\mathcal{J}(\lambda) = -k_BT\ln\left(\sum_X A_{\lambda N}^{N,X}\exp\left[-2XJ/k_BT\right]\right) \quad (8)$$

where we have defined

$$A_Y^{N,X} = \binom{Y-1}{X-1}\binom{N-Y+1}{X}, \quad (9)$$

the number of ways to distribute $Y$ sites in $X$ different domains among $N$ possible sites.

Using Eq. 6, one can then compute the equilibrium number of domains in the zero writhe approximation by numerically determining:

$$X^* = \int dX d\lambda \; X \exp\left[-S_{f,\sigma}(\lambda, X)/k_B T\right] \Big/ \int dX d\lambda \exp\left[-S_{f,\sigma}(\lambda, X)/k_B T\right] \tag{10}$$

In addition, using Eq. 7 and $\langle \bullet \rangle_\lambda \equiv \int d\lambda \bullet \exp\left[-F_{f,\sigma}(\lambda)/k_B T\right] / \int d\lambda \exp\left[-F_{f,\sigma}(\lambda)/k_B T\right]$, one can derive the other equilibrium quantities as follows (see below for torques):

$$\lambda^* = \langle \lambda \rangle_\lambda, \tag{11}$$

$$z^* = -\langle \partial_f F_{f,\sigma}(\lambda) \rangle_\lambda = \lambda^* \epsilon^X + (1 - \lambda^*)\epsilon^B \tag{12}$$

with $\epsilon^s$ the WLC extension associated with the form $s$ of DNA, which depends only on $a_s$ and $\ell_s$ [1].

Note finally that numerical integration is performed by circumventing numerical problems coming from the generation of large combinatorial quantities when $\lambda N$ becomes large (as in the case e.g. of Eq. 9). Recalling that $\lambda = K/N$ where $K$ is the number of sites occupied by the alternative form, the integration thus consists of a discrete sum over restricted values of $K$ and $X$ for which Boltzmann weights are maximal. To this end, we first localise the saddle-point of $S_{f,\sigma}(\lambda, X)$ and then perform the sum over values of $K$ and $X$ lying in the rectangle that contains the saddle-point and outside of which relative Boltzmann weights with respect to the saddle-point are smaller than $10^{-4}$. We further checked that our result did not depend on the choice of this cut-off.

### C. Generalization to an arbitrarily number of alternative forms

In the situation of $k$ possible DNA forms (one B-DNA plus $k-1$ alternative forms), denoting the vector of fraction of each of these forms by $\boldsymbol{\lambda} \equiv \{\lambda_i\}_{i=1..k}$ , with $\sum_{i=1}^k \lambda_i = 1$, the free energy landscape becomes:

$$\mathcal{F}_{f,\sigma}(\boldsymbol{\lambda}) = N_{\rm bp} \sum_{i=1}^k \lambda_i \gamma_i + \mathcal{I}(\boldsymbol{\lambda}) + \sum_{i=1}^k g_{i,f}(\lambda_i N_{\rm bp} a_i) + \frac{k_B T}{2} \left[ \frac{\psi_B^2 N_{\rm bp}}{\sum_{i=1}^k \lambda_i \chi_i} \left(1 + \sigma - \sum_{i=1}^k \lambda_i \frac{\psi_i}{\psi_B}\right)^2 + \ln\left(\sum_{i=1}^k \lambda_i \chi_i\right)\right] \tag{13}$$

where here the index $i$ always indicates the different forms and where $\mathcal{I}(\boldsymbol{\lambda})$ indicates the free energy associated with the multiple possibilities to distribute the different alternative sites into distinct domains.

## D. Torques

### 1. *Measurement in numerical simulations*

To measure the torque exerted by a molecule in our simulations, we use the same method as in our previous work [2] where we adapted a commonly used experimental method [3, 4] to the case of rod-like chain models with global torsional energy. It consists in attaching the ends of the molecule to a reservoir of twists with which this can exchange helix turns. The reservoir, also called a magnetic trap, is characterized by a stiffness $k_R$ such that any variation of the twist within it, $\delta\mathrm{Tw}_R$, with respect to a reference twist (see below) is associated with an energy cost $2\pi^2 k_B T k_R \delta\mathrm{Tw}_R^2$. Similarly to the measurements in magnetic torque tweezers, the equilibrium torque exerted by the molecule is then given by $\Gamma^* = -2\pi k_R(\mathrm{Tw}^* - \mathrm{Tw}_0^*)$, where $\mathrm{Tw}^*$ and $\mathrm{Tw}_0^*$ are respectively the equilibrium twists of the supercoiled molecule and of the corresponding relaxed molecule, both measured in the presence of the magnetic trap. Note here, that the linking number in the reservoir is further calibrated such that $\mathrm{Tw}_0^*$ is equal to the number of helices of the molecule at rest, $\mathrm{Tw}_0$.

### 2. *Expression in the zero writhe approximation and access to the torsional modulus*

The equilibrium torque exerted by the molecule is defined by $\Gamma^* = \langle \partial_\Theta F_{f,\sigma}(\lambda)\rangle_\lambda$ where $\Theta$ is the rotation angle of the tip of the molecule around the stretching direction (the direction perpendicular to the magnetic field used to add helical turns to the molecule). In magnetic tweezers experiments, $\Theta$ is a control parameter related to the linking number: $\Theta = 2\pi\mathrm{Lk}$. As a consequence, $\Gamma^* = (2\pi)^{-1}\langle \partial_{\mathrm{Lk}} F_{f,\sigma}(\lambda)\rangle_\lambda$, which becomes $\Gamma^* = (2\pi\mathrm{Tw}_0)^{-1}\langle \partial_\sigma F_{f,\sigma}(\lambda)\rangle_\lambda$ in the approximation of zero writhe, where $\mathrm{Lk} = \mathrm{Tw}$ and $\sigma = (\mathrm{Tw} - \mathrm{Tw}_0)/\mathrm{Tw}_0$. Using Eq. 7, we thus obtain for the case of the co-existence of X- and B-DNA:

$$\Gamma^* = k_B T \psi_B \left\langle \frac{1 + \sigma - \frac{\psi(\lambda)}{\psi_B}}{\chi(\lambda)} \right\rangle_\lambda \tag{14}$$

We then note that whenever the fraction $\lambda$ of X-DNA is fixed (and known), Eq. 14 can be used to estimate $C_X$ (appearing in $\chi(\lambda)$) by computing the slope of the $\sigma$-torque curve since in this case $\Gamma^* = C^{te} + \frac{k_B T \psi_B}{\chi(\lambda)}\sigma$. This has been used by Bryant's group in the context of small, specifically designed bubble of alternative forms [5, 6].

### E. Inference of parameters by testing a large number of parameters

In the absence of *a priori* knowledge about the mechanical parameters of alternative forms, we used a "blind" approach consisting in i) drawing a large number of points (typically thousands) in the space of parameters according to a uniform distribution, ii) computing $\sigma$-extension curves using the zero-writhe approximation and iii) comparing the generated curves to the original data (either simulated data as in Figure 4 of the main text or experimental data as in Figure 5 of the main text). To limit the space of parameters, we made $a$ vary between 0.34 nm (B-DNA) and 0.7 nm (approximately the largest value measured for denatured DNA before breaking [7]), $\ell$ vary between 1 nm (lowest estimate for denatured DNA [8]) and 15 nm (at least 5 times larger than any previous estimations for either D-DNA or L-DNA), $C$ vary between 1 nm (lowest estimate of both D-DNA and L-DNA [8]) and 100 nm (typical value for B-DNA), $\psi$ vary between -0.6 and 0.6 rad/bp (helicity of B-DNA), $\gamma$ vary between 1 $k_BT$ and 3 $k_BT$ (the average free energy formation cost of alternative forms is estimated to be around 2 $k_BT$ [9]) and $J$ vary between 2 $k_BT$ (leading to several domains in our simulations) and 20 $k_BT$ (single domain).


[1] R. Strick, M.-N. Dessinges, G. Charvin, N. H. Dekker, J.-F. Allemand, D. Bensimon, and V. Croquette, "Stretching of macromolecules and proteins," Reports on Progress in Physics **66**, 1–45 (2003).

[2] Thibaut Lepage, François Képès, and Ivan Junier, "Thermodynamics of Long Supercoiled Molecules: Insights from Highly Efficient Monte Carlo Simulations." Biophysical Journal **109**, 135–143 (2015).

[3] László Oroszi, Péter Galajda, Huba Kirei, Sándor Bottka, and Pál Ormos, "Direct measurement of torque in an optical trap and its application to double-strand DNA." Physical Review Letters **97**, 058301 (2006).

[4] Jan Lipfert, Jacob W J. Kerssemakers, Tessa Jager, and Nynke H. Dekker, "Magnetic torque tweezers: measuring torsional stiffness in DNA and RecA-DNA filaments." Nat Methods **7**, 977–980 (2010).

[5] Florian C Oberstrass, Louis E Fernandes, and Zev Bryant, "Torque measurements reveal sequence-specific cooperative transitions in supercoiled DNA." Proceedings of the National Academy of Sciences **109**, 6106–6111 (2012).

[6] F C Oberstrass, L E Fernandes, P Lebel, and Z Bryant, "Torque Spectroscopy of DNA: Base-Pair Stability, Boundary Effects, Backbending, and Breathing Dynamics," Physical Review Letters (2013).

[7] D. Bensimon, A. J. Simon, V. Croquette, and A. Bensimon, "Stretching DNA with a Receding Meniscus: Experiments and Models," Phys. Rev. Lett. **74**, 4754–4757 (1995).

[8] Maxim Y Sheinin, Scott Forth, John F Marko, and Michelle D Wang, "Underwound DNA under Tension: Structure, Elasticity, and Sequence-Dependent Behaviors," Physical Review Letters **107**, 108102 (2011).

[9] J SantaLucia, "A unified view of polymer, dumbbell, and oligonucleotide DNA nearest-neighbor thermodynamics." Proceedings of the National Academy of Sciences of the United States of America **95**, 1460–1465 (1998).

## II. SUPPLEMENTARY FIGURES

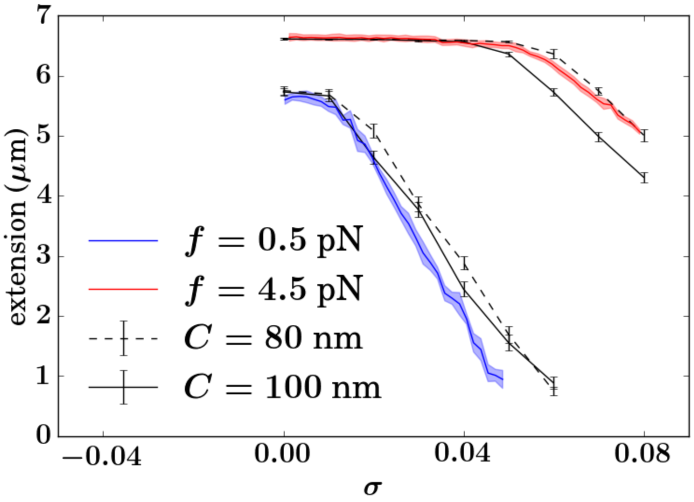


FIG. S1. Effect of $C$ on the simulated extension curves. Using $C = 100\,\text{nm}$ fits better the experimental data for $f = 0.5\,\text{pN}$ while $C = 80\,\text{nm}$ gives a better agreement for $f = 4.5\,\text{pN}$.

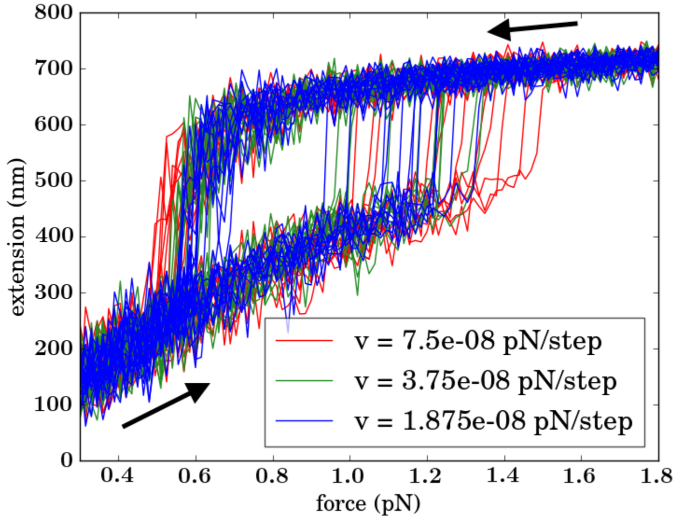


FIG. S2. Hysteresis cycles around the plectonemic-denatured transition. Simulations of a 2.4 kb molecule were performed ($\sigma = -0.05$) during which the force was continuously increased (as indicated by the lower left arrow) and decreased (upper right arrow arrow) at constant speed from 0.3 to 1.8 pN. For each of the three speeds reported here (from the fastest to the slowest: red, green and blue curves), 12 cycles were performed, revealing in each case a strong hysteresis pattern in the force-extension diagram.

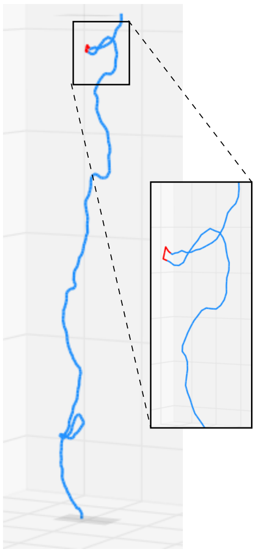

FIG. S3. Snapshot of a simulation close to the plectoneme-denaturation transition (in the figure S2). A denaturation bubble (red) appears at the apex of a plectoneme.

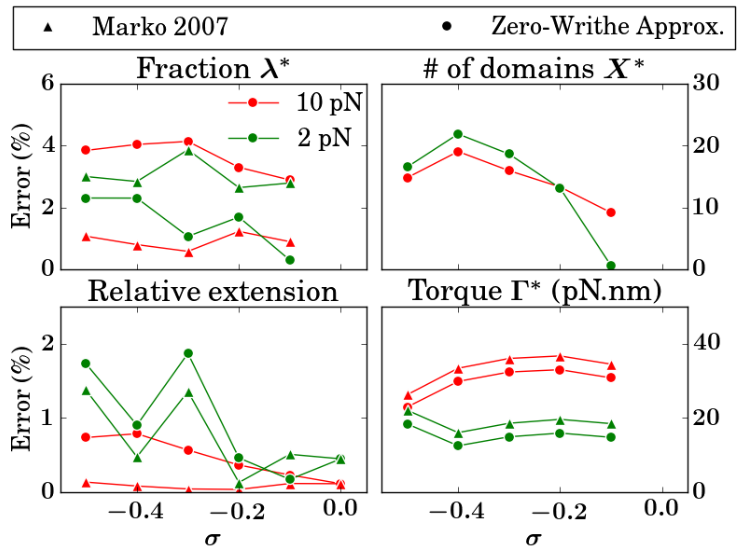


FIG. S4. Relative difference between the zero-writhe approximation and our simulations and between Marko's model and our simulations, corresponding to Fig. 3 in the main text.

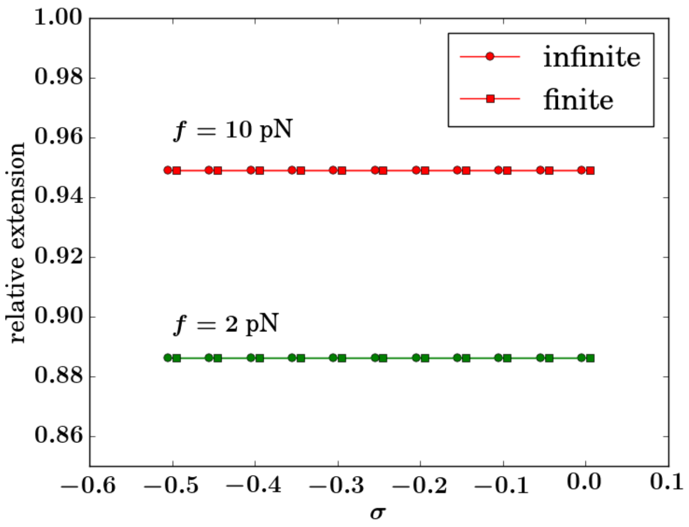


FIG. S5. FInite-size effects on the zero-writhe approximation: extension as a function of $\sigma$ for 2 different forces, including finite-size effects (squares) or not (circles). The points are actually almost exactly superimposed; they were slightly offset along the x-axis for readability.

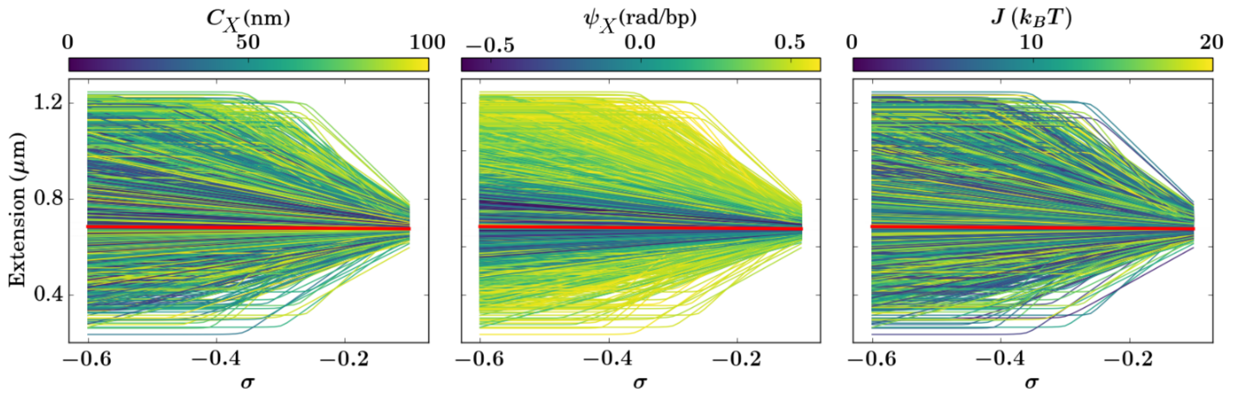


FIG. S6. Rainbow plots of the extension with respect to the varying parameters not shown in Fig.3 of the main text, namely, $C_X$, $\psi_X$ and $J$. $C_X$ and $J$ have no effect on the extension. For $\psi_X$, values away from $\psi_B = 0.6\,\text{rad/bp}$ tend to yield better fits.

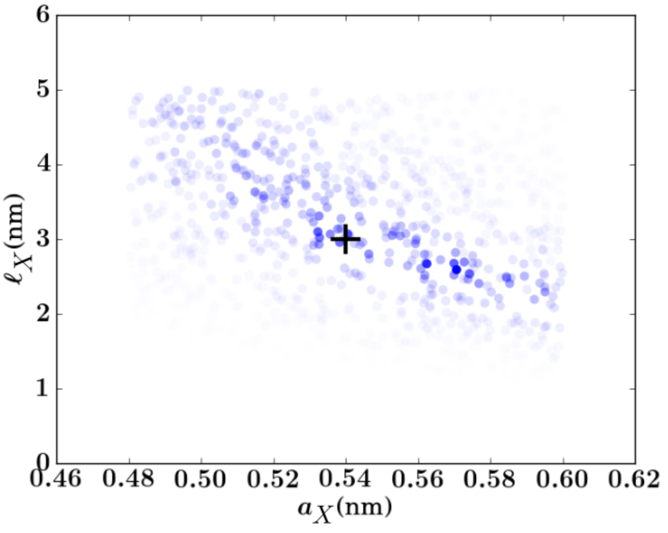


FIG. S7. In a situation where $\psi = \hat{\psi}_X$ and $C = \hat{C}_X$, combining RMSDs for multiple forces $(2, 2.5, 3, 3.5, 6, 8.5$ and $12\,\text{pN})$, the best solutions resulting from the intersection of the crests shown in Fig. 2 of the main text are located around $(\hat{a}_X, \hat{\ell}_X)$ (black cross).

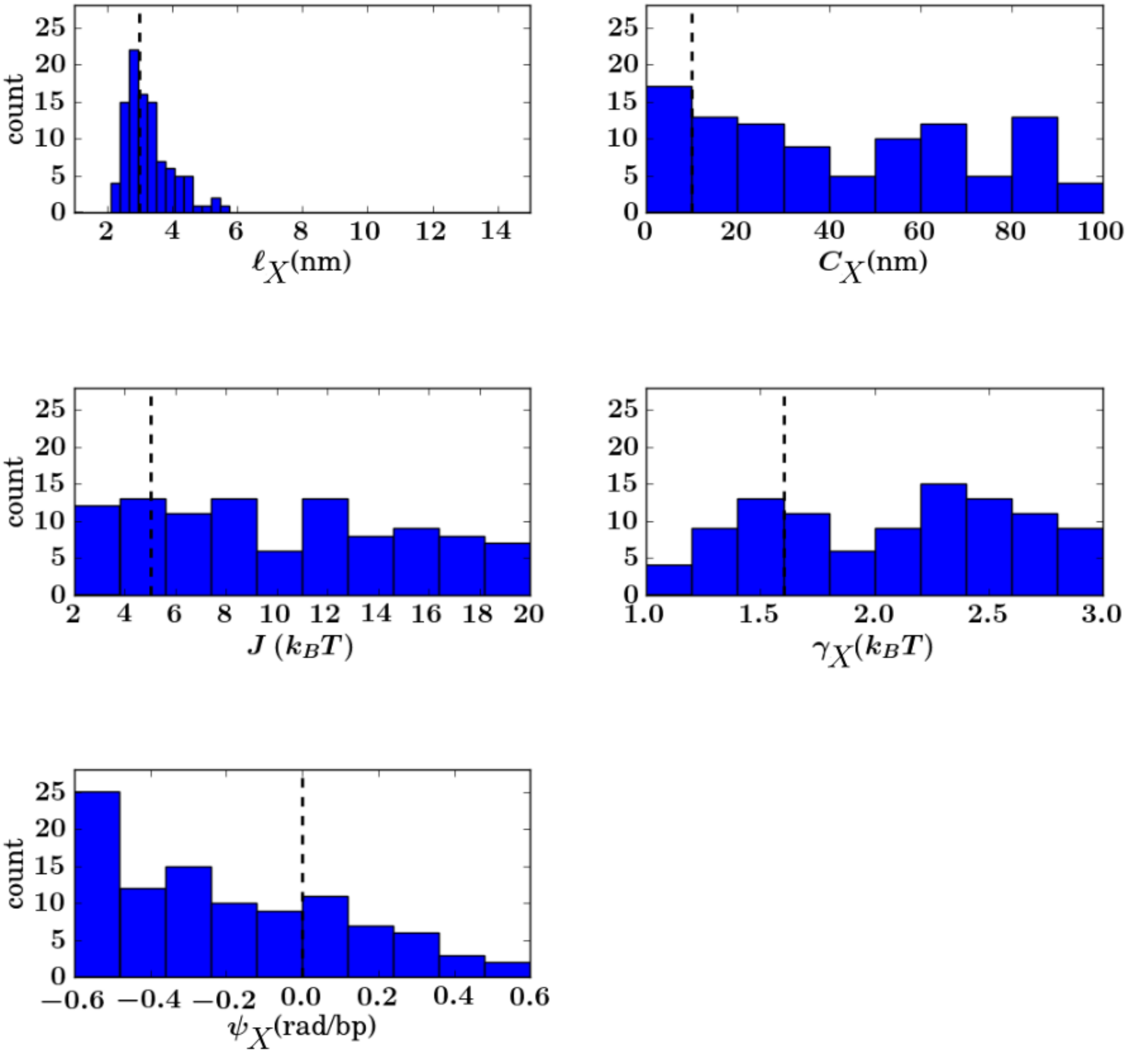


FIG. S8. Typical values of parameters for best fit solutions. Within the slice $a_X \in [0.52, 0.56\,\text{nm}]$ centered around $\hat{a}_X$ (see Fig. 4 in the main article), we selected the 100 best fits to the fake data and plotted the histogram of values for the other parameters (dashed lines represent $\hat{\ell}_X, \hat{C}_X, \hat{J}$ and $\hat{\gamma}_X$). Contrary to the other parameters that spread across all their allowed range, the values of $\ell_X$ are concentrated around $\hat{\ell}_X$ (top left).

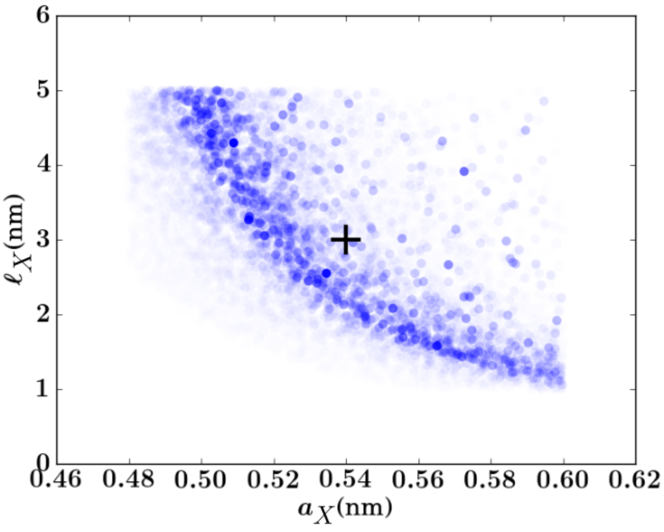


FIG. S9. Setting only $\psi_X = \hat{\psi}_X$ $(= 0)$, at high force (12 pN) we find a crest of sub-optimal fits that go off the original parameters $(\hat{a}_X, \hat{\ell}_X)$ (black cross).

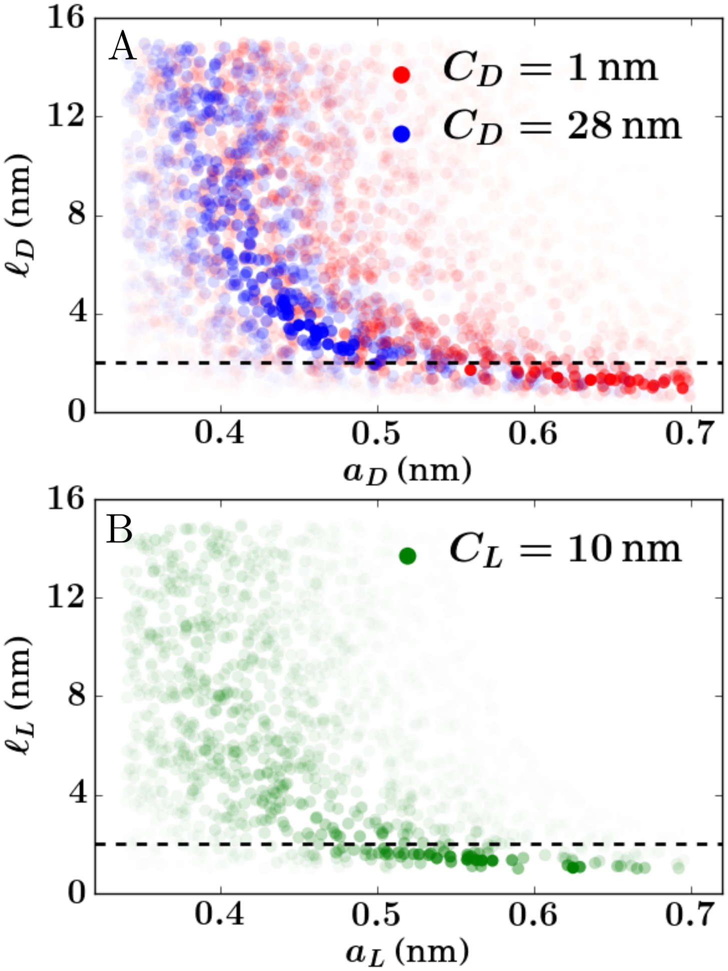


FIG. S10. Effect of the coarse-graining on the zero-writhe approximation. The results of Fig. 5 of the main text are unchanged when using a different level of discretization (here $n = 4$).

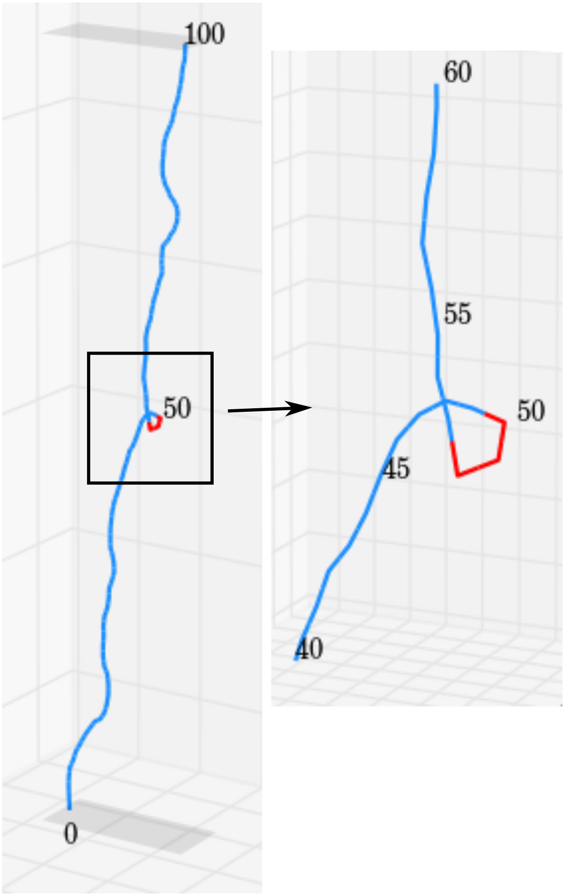


FIG. S11. Snapshot of a simulation of a 1 kb-long molecule (100 cylinders, $f = 1\,\mathrm{pN}$, $\sigma = -0.06$) where the cylinder at the center (number 50) has no denaturation penalty ($\gamma_{D,i=50} = 0$). The denaturation bubble (red) appears and stays at the center during the whole simulation.
